# Supplementary material for: Not All Actions Are Created Equal: Bayesian Optimal Experimental Design for Safe and Optimal Nonlinear System Identification
Source: arXiv:2308.01829 source file (2023-08-03)
Supplement: Supplementary file 1 [file 09_Appendix.tex]

\section{Proof of Proposition 17}
\label{app:prop}

\begin{proof}
To compute (12) we approximate the integral using cubature.
Thus, we compute the $N$ cubature weights and points, $w_i$ and $\theta_i$ respectively, for the sample space $\Theta$.
From (11) the measurement likelihood conditioned on $\theta$ is a Gaussian distribution whose mean is a function of $\theta$.
The initial state of the system, $x_0$ is known given Assumption 8, and we compute the mean $g(x(t;k, \theta_i))$ of the measurement likelihood given the cubature samples $\theta_i$.

Then

\begin{align}
    p(y; k) &= \frac{1}{Z} \sum_{i=1}^N w_i p(y \mid \theta_i) p(\theta_i) \\
    &= \frac{1}{Z} \sum_{i=1}^N w_i p(\theta_i) \N(g(x(t;k,\theta_i)), \Sigma)
\end{align}

\noindent where $Z = \sum_{l=1}^N w_l p(\theta_l)$ is the normalizing constant.

\end{proof}

\section{Proof for Corollary 19} \label{app:cor}

\begin{proof}
    Per Proposition 17 the measurement marginal is approximated as a Gaussian Mixture Model.
    The Kullbeck-Leibler divergence between the Gaussian measurement likelihood and measurement marginal, (19), is lower-bounded using Jensen's inequality as (12) in [29].
    Thus we arrive at (24).
\end{proof}

\section{Tire Forces for Vehicle Model} \label{appendix:tire_forces}

We assume the vehicle with dynamics specified in (31) is front-wheel drive, thus the longitudinal rear tire forces are zero $F_\text{xr}(t) = 0$.
The lateral rear tire forces are treated as an observable

\begin{equation}
    F_\text{yr}(t) = \Bar{c}_{\alpha r} \alpha_r(t)
\end{equation}

\noindent where $\Bar{c}_{\alpha r}$ is the cornering stiffness for the rear tires and $\alpha_r(t)$ is the slip angle

\begin{equation}
    \alpha_r(t) = -\frac{x_5(t) - l_r x_6(t)}{x_4(t)}
\end{equation}

The longitudinal front tire force with user-chosen constants $K_u,\kappa_{1,u},\kappa_{2,u},\phi_{1,u},\phi_{2,u}\in\R_+$ is computed as

\begin{equation}
    \label{eq: Fxf}
    \begin{split}
    F_\text{xf}(t;k) = -m K_u (x_4(t) - \xdes_4(t;k) ) + m\dxdes_4(t;k) + \\ - F_\text{xr}(t;k)- m x_5(t) x_6(t) + m\tau_u(t;k)
    \end{split}
\end{equation}

\noindent where 

\begin{align}
    \tau_u(t;k) =& -\big(\kappa_u(t;k) M_u+\phi_u(t;k)\big)e_u(t;k), \label{eq: tau_u def} \\
    \kappa_u(t;k) =& \kappa_{1,u}+\kappa_{2,u}\int_{\tz}^t\|x_4(s)-\xdes_4(s;k)\|^2ds,\label{eq: kappa_u def}\\
    \phi_u(t;k) =&\phi_{1,u}+\phi_{2,u}\int_{\tz}^t\|x_4(s)-\xdes_4(s;k)\|^2ds,\label{eq: phi_u def}\\
    e_u(t;k) =& x_4(t)-\xdes_4(t;k) \label{eq: e_u def}
\end{align}

The lateral front tire force with user-chosen constants $K_h,K_r,\kappa_{1,r},\kappa_{2,r},\phi_{1,r},\phi_{2,r}\in\R_+$ are computed as

\begin{equation}
\label{eq: Fyf}
\begin{split}
     F_\text{yf}(t;k) = -\frac{I_\text{zz} K_r}{l_\text{f}}\left( x_6(t) - \xdes_6(t;k) \right) +  \frac{I_\text{zz}}{l_\text{f}} \dxdes_6(t;k) + \\ -\frac{I_\text{zz} K_h}{l_\text{f}}\left( x_3(t) - \xdes_3(t;k)\right) + \frac{l_\text{r}}{l_\text{f}} F_\text{yr}(t) + \frac{I_\text{zz}}{l_\text{f}} \tau_r(t;k),
     \end{split}
\end{equation}

\noindent where

\begin{align}
 \tau_r(t;k) =& -\big(\kappa_r(t;k) M_r+\phi_r(t;k)\big)e_r(t;k) \label{eq: tau_r def} \\
    \kappa_r(t;k) =& \kappa_{1,r}+\kappa_{2,r}\int_{\tz}^t\left\| \begin{bmatrix}x_6(s)\\x_3(s)\end{bmatrix} - \begin{bmatrix}\xdes_6(s;k)\\\xdes_3(s;k)\end{bmatrix}\right\|^2ds\\
    \phi_r(t;k) =&\phi_{1,r}+\phi_{2,r}\int_{\tz}^t\left\| \begin{bmatrix}x_6(s)\\x_3(s)\end{bmatrix} - \begin{bmatrix}\xdes_6(s;k)\\\xdes_3(s;k)\end{bmatrix}\right\|^2ds\\
    e_r(t;k) =& \begin{bmatrix} K_r & K_h \end{bmatrix} \begin{bmatrix} x_6(t)-\xdes_6(t;k) \\ x_3(t)-\xdes_3(t;k) \end{bmatrix}
\end{align}

\section{Vehicle Parameter Values} \label{app:veh_param}

\section{Modified Vehicle Dynamics} \label{appendix:mod_veh_dyn}

We describe how to compute the tire forces for the baseline comparison [8] given input parameters $\delta$ and $\omega(t)$ corresponding to the steering angle and the front tire rotation speed, respectively.
As the vehicle is front-wheel drive, the rear longitudinal tire force is $0$N.
The front longitudinal tire force is computed as

\begin{equation}
    F_{xf}(t) = \frac{m g l_r}{l} \mu \lambda(t)
\end{equation}

\noindent where $\mu$ is a constant, $r_w$ is the tire radius, $\omega_i(t)$ is the tire-rotation speed at time $t$, and

\begin{equation}
    \lambda(t) = \begin{cases}
        \frac{r_w \omega(t) - x_4(t)}{x_4(t)} & \mbox{if braking} \\
        \frac{r_w \omega(t) - x_4(t)}{r_w \omega(t)} & \mbox{if accelerating}
    \end{cases}
\end{equation}

For the low-speed vehicle dynamics the lateral tire forces are not computed.

\section{Trajectory Parameterization for Autonomous Vehicle}

We use two parameters, $k = [k_1, k_2] \in \K$, to parameterize the vehicle's trajectory.
The lane change and turning maneuvers include both a driving and braking phase, where per Assumption 9, the braking phase ensures the vehicle can come to a stop safely without colliding with obstacles.
We specify the duration for each driving phase $t_m$, a duration for the braking phase $t_b$, and the time when the vehicle has come to a stop $t_s = t_m + t_b$.

For the lane change maneuver, we parameterize the desired longitudinal speed and heading of the vehicle as

\begin{equation}
    x_3^{des}(t,k) = \begin{cases}
        x_3(0) + h_1 k_2 \exp\big(-h_2 (t - 0.5 t_b)^2 \big), \\
        \qquad \qquad \qquad \qquad, \text{ if } 0 < t < t_b \\
        x_3(0), \; \; \quad \qquad \qquad  \text{ if } t \geq t_b
    \end{cases}
\end{equation}

\begin{equation}
    x_4^{des}(t,k) = \begin{cases}
        x_4(0) + \frac{k_1 - x_4(0)}{t_{m}} t, \quad \text{if } 0 < t < t_{m} \\
        x_4^{brake}(t,k), \quad \quad \; \; \; \quad \text{if } t > t_{m} \\
    \end{cases}
\end{equation}

\noindent where $h_1$ and $h_2$ are user-specified constants used to adjust the amplitude of the lane change maneuver, and

\begin{equation} \label{eq:speed_brake}
    x_4^{brake}(t,k) = \begin{cases}
        k_1 + (t - t_m) a^{decel}, \\
        \quad \quad \quad \text{, if } k_1 > x_4^{crit} \text{ and } t_{b} < t < t_s \\
        0, \quad \quad \; \text{ if } k_1 > x_4^{crit} \text{ and } t \geq t_s \\
        0, \quad \quad \; \text{ if } k_1 \leq x_4^{crit} \text{ and } t \geq t_s \\
    \end{cases}
\end{equation}

For the left turning maneuver, we parameterize the longitudinal speed and yaw rate of change as

\begin{equation}
    x_4^{des}(t,p) = \begin{dcases}
        \frac{11}{2}t,      \hspace{1.15cm} \text{ if } 0\leq t<\frac{1}{4}\tm \text{ and } \frac{11}{8}\tm< p_u\\
        k_1,        \hspace{1.35cm} \text{ if } 0\leq t<\frac{1}{4}\tm \text{ and } \frac{11}{8}\tm\geq p_u\\
        k_1,       \hspace{1.35cm} \text{ if } \frac{1}{4}\tm\leq t<\tm\\
        x_4^{brake}(t,p),\hspace{0.2cm} \text { if } t\geq\tm
    \end{dcases}
\end{equation}

\begin{equation}
    x_6^{des}(t,p) = \begin{dcases}
        \frac{1}{2} k_2 \left(1-\cos\left(\frac{4\pi}{\tm} t\right)\right),      \hspace{0.1cm} \text{ if } 0\leq t<\frac{1}{4}\tm\\
        k_2,       \hspace{3.25cm} \text{ if } \frac{1}{4}\tm\leq t<\frac{3}{4}\tm\\
        \frac{1}{2} k_2 \left(1-\cos\left(\frac{4\pi}{\tm} t\right)\right),      \hspace{0.1cm} \text{ if } \frac{3}{4}\tm\leq t<\tm\\
        0,\hspace{3.42cm} \text { if } t\geq\tm
    \end{dcases}
\end{equation}

\noindent where $x_4^{brake}$ is computed as \eqref{eq:speed_brake}.

The driving maneuver time $\tm$ is set at 6 seconds for the lane change maneuver and 4 seconds for the turning maneuver.
The planning time $\tplan$ is set as 3 seconds.

For the lane change and turning maneuver the time required for the braking phase, $t_b$, is a function of the vehicle's velocity, a constant deceleration $a^{deccel} < 0$, and a critical longitudinal speed $x_4^{crit}$ at which the system switches from high-speed to low-speed dynamics.
We compute the braking phase time as

\begin{equation}
    t_b = \begin{cases}
        1.5 + \frac{x_4^{crit} - k_1}{a^{decel}}, \hspace{0.1cm} \text{ if } k_1 > x_4^{crit} \\
        1.5, \hspace{1.7cm} \text{ if } k_1 \leq x_4^{crit}
    \end{cases}.
\end{equation}
